# Supplementary material for: An Efficient Self-Supervised Cross-View Training For Sentence Embedding
Source: arXiv:2311.03228 source file (2023-11-06)
Supplement: Supplementary file 1 [file 7_appendix.tex]

\appendix
\section{Appendix}

\subsection{Temperature Scaling}
\label{appendix:temperature}
In this study, we show performance changing when we change the temperature scaling number.
We tested on BERT-Tiny and MiniLM-L3 across seven STS benchmark datasets.

As shown in Table~\ref{tab:temperature_stuides} and Table~\ref{tab:temperature_stuides_2}, we highlight the performance change with heat map. 
The best range of these models are $\tau^\theta$ equal to 0.03 to 0.04 and $\tau^\text{ref}$ equal to 0.01 to 0.04 on both models.
In addition, the number near the best setting also demonstrates the same performance. 

\begin{table}[h]
% \vspace{-3mm}

\centering
\setlength\doublerulesep{3pt}
\scalebox{0.7}{
\setlength{\tabcolsep}{3.5pt}
%\fontsize{10pt}{12pt}\selectfont
\begin{tabular}{cc|ccccccc|}
\cline{3-9}
\multicolumn{2}{l|}{} &
  \multicolumn{7}{c|}{\textbf{$\tau^\theta$}} \\ \cline{3-9} 
\multicolumn{2}{l|}{\multirow{-2}{*}{\textbf{}}} &
  \multicolumn{1}{c|}{0.01} &
  \multicolumn{1}{c|}{0.02} &
  \multicolumn{1}{c|}{0.03} &
  \multicolumn{1}{c|}{0.04} &
  \multicolumn{1}{c|}{0.05} &
  \multicolumn{1}{c|}{0.07} &
  0.1 \\ \hline
\multicolumn{1}{|c|}{} &
  0.01 &
  \multicolumn{1}{c|}{\cellcolor[HTML]{F2B7B2}64.40} &
  \multicolumn{1}{c|}{\cellcolor[HTML]{EB938C}67.64} &
  \multicolumn{1}{c|}{\cellcolor[HTML]{E8827A}69.18} &
  \multicolumn{1}{c|}{\cellcolor[HTML]{EA918A}67.84} &
  \multicolumn{1}{c|}{\cellcolor[HTML]{EDA09A}66.45} &
  \multicolumn{1}{c|}{\cellcolor[HTML]{F1B1AC}64.88} &
  \cellcolor[HTML]{F0B0AB}64.98 \\ \cline{2-9} 
\multicolumn{1}{|c|}{} &
  0.02 &
  \multicolumn{1}{c|}{\cellcolor[HTML]{EDA09A}66.44} &
  \multicolumn{1}{c|}{\cellcolor[HTML]{EA8E86}68.10} &
  \multicolumn{1}{c|}{\cellcolor[HTML]{E98981}68.57} &
  \multicolumn{1}{c|}{\cellcolor[HTML]{E8847C}69.02} &
  \multicolumn{1}{c|}{\cellcolor[HTML]{ED9C96}66.81} &
  \multicolumn{1}{c|}{\cellcolor[HTML]{F1B6B1}64.49} &
  \cellcolor[HTML]{F2B8B4}64.23 \\ \cline{2-9} 
\multicolumn{1}{|c|}{} &
  0.03 &
  \multicolumn{1}{c|}{\cellcolor[HTML]{EC9992}67.12} &
  \multicolumn{1}{c|}{\cellcolor[HTML]{EA9089}67.91} &
  \multicolumn{1}{c|}{\cellcolor[HTML]{E8877E}68.81} &
  \multicolumn{1}{c|}{\cellcolor[HTML]{E67C73}\textbf{69.73}} &
  \multicolumn{1}{c|}{\cellcolor[HTML]{EB968F}67.35} &
  \multicolumn{1}{c|}{\cellcolor[HTML]{F5C6C2}62.99} &
  \cellcolor[HTML]{FAE3E1}60.35 \\ \cline{2-9} 
\multicolumn{1}{|c|}{} &
  0.04 &
  \multicolumn{1}{c|}{\cellcolor[HTML]{EA8D85}68.25} &
  \multicolumn{1}{c|}{\cellcolor[HTML]{EA8D85}68.19} &
  \multicolumn{1}{c|}{\cellcolor[HTML]{E8847C}69.00} &
  \multicolumn{1}{c|}{\cellcolor[HTML]{E8877E}68.79} &
  \multicolumn{1}{c|}{\cellcolor[HTML]{EEA39D}66.20} &
  \multicolumn{1}{c|}{\cellcolor[HTML]{F6CCC9}62.39} &
  \cellcolor[HTML]{FDF0EF}59.15 \\ \cline{2-9} 
\multicolumn{1}{|c|}{} &
  0.05 &
  \multicolumn{1}{c|}{\cellcolor[HTML]{E98C84}68.35} &
  \multicolumn{1}{c|}{\cellcolor[HTML]{EA9089}67.92} &
  \multicolumn{1}{c|}{\cellcolor[HTML]{EC9992}67.13} &
  \multicolumn{1}{c|}{\cellcolor[HTML]{ED9F98}66.61} &
  \multicolumn{1}{c|}{\cellcolor[HTML]{ED9D96}66.78} &
  \multicolumn{1}{c|}{\cellcolor[HTML]{F5C9C5}62.69} &
  \cellcolor[HTML]{FCF0EE}59.17 \\ \cline{2-9} 
\multicolumn{1}{|c|}{} &
  0.07 &
  \multicolumn{1}{c|}{\cellcolor[HTML]{FFFFFF}57.71} &
  \multicolumn{1}{c|}{\cellcolor[HTML]{F7D5D2}61.59} &
  \multicolumn{1}{c|}{\cellcolor[HTML]{F6CBC8}62.50} &
  \multicolumn{1}{c|}{\cellcolor[HTML]{F5CAC6}62.63} &
  \multicolumn{1}{c|}{\cellcolor[HTML]{F4C6C2}63.00} &
  \multicolumn{1}{c|}{\cellcolor[HTML]{F3BEBA}63.71} &
  \cellcolor[HTML]{F4C5C1}63.10 \\ \cline{2-9} 
\multicolumn{1}{|c|}{\multirow{-7}{*}{\textbf{$\tau^\text{ref}$}}} &
  0.1 &
  \multicolumn{1}{c|}{\cellcolor[HTML]{FCEDEB}59.45} &
  \multicolumn{1}{c|}{\cellcolor[HTML]{F8D6D4}61.48} &
  \multicolumn{1}{c|}{\cellcolor[HTML]{F4C5C1}63.10} &
  \multicolumn{1}{c|}{\cellcolor[HTML]{F3BEBA}63.70} &
  \multicolumn{1}{c|}{\cellcolor[HTML]{F3BDB9}63.80} &
  \multicolumn{1}{c|}{\cellcolor[HTML]{F3BCB7}63.91} &
  \cellcolor[HTML]{F2BAB6}64.05 \\ \hline
\end{tabular}}
% \vspace{-2mm}
\caption{\label{font-table} Ablation studies on the online temperature $\tau^\theta$ and the target temperature $\tau^\text{ref}$ of BERT-Tiny. We evaluate the average Spearman's correlation on seven STS datasets.}
\vspace{-3mm}
\label{tab:temperature_stuides}
\end{table}
\begin{table}[h]
% \vspace{-3mm}

\centering
\setlength\doublerulesep{3pt}
\scalebox{0.7}{
\setlength{\tabcolsep}{3.5pt}
%\fontsize{10pt}{12pt}\selectfont
\begin{tabular}{cc|ccccccc|}
\cline{3-9}
\multicolumn{2}{l|}{} &
  \multicolumn{7}{c|}{\textbf{$\tau^\theta$}} \\ \cline{3-9} 
\multicolumn{2}{l|}{\multirow{-2}{*}{}} &
  \multicolumn{1}{c|}{0.01} &
  \multicolumn{1}{c|}{0.02} &
  \multicolumn{1}{c|}{0.03} &
  \multicolumn{1}{c|}{0.04} &
  \multicolumn{1}{c|}{0.05} &
  \multicolumn{1}{c|}{0.07} &
  0.1 \\ \hline
\multicolumn{1}{|c|}{} &
  0.01 &
  \multicolumn{1}{c|}{\cellcolor[HTML]{ED9C96}64.57} &
  \multicolumn{1}{c|}{\cellcolor[HTML]{EA8F88}66.90} &
  \multicolumn{1}{c|}{\cellcolor[HTML]{E98C84}67.57} &
  \multicolumn{1}{c|}{\cellcolor[HTML]{E98A82}67.84} &
  \multicolumn{1}{c|}{\cellcolor[HTML]{E98B83}67.62} &
  \multicolumn{1}{c|}{\cellcolor[HTML]{EDA099}63.91} &
  \cellcolor[HTML]{ED9D96}64.50 \\ \cline{2-9} 
\multicolumn{1}{|c|}{} &
  0.02 &
  \multicolumn{1}{c|}{\cellcolor[HTML]{EB948D}66.03} &
  \multicolumn{1}{c|}{\cellcolor[HTML]{E98A82}67.79} &
  \multicolumn{1}{c|}{\cellcolor[HTML]{EA8F87}66.94} &
  \multicolumn{1}{c|}{\cellcolor[HTML]{E8857D}68.72} &
  \multicolumn{1}{c|}{\cellcolor[HTML]{E98981}68.01} &
  \multicolumn{1}{c|}{\cellcolor[HTML]{EA9189}66.64} &
  \cellcolor[HTML]{ED9D96}64.42 \\ \cline{2-9} 
\multicolumn{1}{|c|}{} &
  0.03 &
  \multicolumn{1}{c|}{\cellcolor[HTML]{EB948D}66.05} &
  \multicolumn{1}{c|}{\cellcolor[HTML]{EA8F87}66.96} &
  \multicolumn{1}{c|}{\cellcolor[HTML]{E8847C}68.85} &
  \multicolumn{1}{c|}{\cellcolor[HTML]{E67C73}\textbf{70.16}} &
  \multicolumn{1}{c|}{\cellcolor[HTML]{E8877F}68.41} &
  \multicolumn{1}{c|}{\cellcolor[HTML]{EC9790}65.54} &
  \cellcolor[HTML]{EEA59F}63.06 \\ \cline{2-9} 
\multicolumn{1}{|c|}{} &
  0.04 &
  \multicolumn{1}{c|}{\cellcolor[HTML]{EB928A}66.47} &
  \multicolumn{1}{c|}{\cellcolor[HTML]{EB958E}65.91} &
  \multicolumn{1}{c|}{\cellcolor[HTML]{EA8F87}67.04} &
  \multicolumn{1}{c|}{\cellcolor[HTML]{E8857C}68.83} &
  \multicolumn{1}{c|}{\cellcolor[HTML]{E98981}68.09} &
  \multicolumn{1}{c|}{\cellcolor[HTML]{EC9B94}64.82} &
  \cellcolor[HTML]{F3BBB7}58.98 \\ \cline{2-9} 
\multicolumn{1}{|c|}{} &
  0.05 &
  \multicolumn{1}{c|}{\cellcolor[HTML]{EA8E86}67.21} &
  \multicolumn{1}{c|}{\cellcolor[HTML]{EB938C}66.23} &
  \multicolumn{1}{c|}{\cellcolor[HTML]{EA9088}66.83} &
  \multicolumn{1}{c|}{\cellcolor[HTML]{EA8C84}67.46} &
  \multicolumn{1}{c|}{\cellcolor[HTML]{EA8C85}67.42} &
  \multicolumn{1}{c|}{\cellcolor[HTML]{EEA6A0}62.80} &
  \cellcolor[HTML]{F5C7C3}57.00 \\ \cline{2-9} 
\multicolumn{1}{|c|}{} &
  0.07 &
  \multicolumn{1}{c|}{\cellcolor[HTML]{FAE5E3}51.60} &
  \multicolumn{1}{c|}{\cellcolor[HTML]{F9DFDD}52.59} &
  \multicolumn{1}{c|}{\cellcolor[HTML]{F9DFDD}52.63} &
  \multicolumn{1}{c|}{\cellcolor[HTML]{F9DDDB}52.91} &
  \multicolumn{1}{c|}{\cellcolor[HTML]{F8D8D6}53.79} &
  \multicolumn{1}{c|}{\cellcolor[HTML]{F8D7D5}53.98} &
  \cellcolor[HTML]{FFFEFE}46.99 \\ \cline{2-9} 
\multicolumn{1}{|c|}{\multirow{-7}{*}{\textbf{$\tau^\text{ref}$}}} &
  0.1 &
  \multicolumn{1}{c|}{\cellcolor[HTML]{FCEDEC}50.13} &
  \multicolumn{1}{c|}{\cellcolor[HTML]{FCEBEA}50.41} &
  \multicolumn{1}{c|}{\cellcolor[HTML]{FAE2E0}52.04} &
  \multicolumn{1}{c|}{\cellcolor[HTML]{FFFFFF}46.78} &
  \multicolumn{1}{c|}{\cellcolor[HTML]{FBE8E6}51.04} &
  \multicolumn{1}{c|}{\cellcolor[HTML]{FCEDEC}50.03} &
  \cellcolor[HTML]{FDF3F2}49.11 \\ \hline
\end{tabular}}
% \vspace{-2mm}
\caption{\label{font-table} Ablation studies on the online temperature $\tau^\theta$ and the target temperature $\tau^\text{ref}$ of MiniLM-L3. We evaluate the average Spearman's correlation on seven STS datasets.}
\vspace{-3mm}
\label{tab:temperature_stuides_2}
\end{table}

\subsection{Ablation Studies Explanation}
\label{appendix:full_ablations}
We describe the implementation details of each ablation study (Table~\ref{tab:ablation_stuides}) as follows:
\begin{compactitem}[\hspace{\setalign}•]
    \item \emph{$f_\text{ref}\rightarrow$ a momentum encoder}. We replace $f_\text{ref}$ with an exponential moving average (EMA) and update the momentum model every iteration follow \citet{DBLP:conf/cvpr/He0WXG20}. 
    \item \emph{KL$\rightarrow$CE}. We change the distribution minimization from KL-divergence to cross-entropy.
    \item \emph{Distribution$\rightarrow$Contrastive}. We let the online encoder learns the representation following the contrastive learning paradigm from MoCo~\cite{DBLP:conf/cvpr/He0WXG20}.
    \item \emph{No MLPs}. We remove MLPs $h(\cdot)$ from our learning pipeline. 
    \item \emph{Cross-view$\rightarrow$Identical-view}. We change how we formulate the similarity distribution as follows:  $c^{\text{on1}} = \mathbf{SR}(z^{\text{on1}}, \mathbf{D}^{1}, \tau^{\theta})$ and  $c^{\text{on2}} = \mathbf{SR}(z^{\text{on2}}, \mathbf{D}^{2}, \tau^{\theta})$. In addition, the reference distribution is still the same.
    \item \emph{Only one instance queue}. Instead of having two instance queues, we combine two queues into one queue where the queue size is $2k$. 
    \item \emph{No update queues}. After randomly generating the queues, we do not update the representation in the queue. 
    \item \emph{No instance queues}. We remove instance queues from our training pipeline. 
    \item \emph{Masked language model}. We random replace 15\% of words in a sentence with [MASK] and replacing with BERT-Base.
    \item \emph{Synonym replacement}. We random replace one word in a sentence with a synonym word. 
    \item \emph{Dropout mask}. We use only transformer dropout mask similar to \citet{gao-etal-2021-simcse}.
    \item \emph{Using the same BT}. We only use the same augmentation for both view inputs. 
\end{compactitem}
